# Supplementary material for: Reinforcement Learning with Videos: Combining Offline Observations with Interaction
Source: arXiv:2011.06507 source file (2021-11-04)
Supplement: Supplementary file 1 [file paired_data_appendix.tex]

\begin{figure}
\newcommand{\pairwidth}{0.11\linewidth}
    \centering
    \includegraphics[width=\pairwidth]{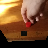}
    \includegraphics[width=\pairwidth]{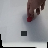}
    \includegraphics[width=\pairwidth]{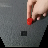}
    \includegraphics[width=\pairwidth]{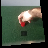}
    \includegraphics[width=\pairwidth]{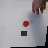}
    \includegraphics[width=\pairwidth]{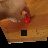}
    \includegraphics[width=\pairwidth]{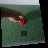}
    \includegraphics[width=\pairwidth]{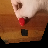}

    \includegraphics[width=\pairwidth]{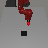}
    \includegraphics[width=\pairwidth]{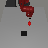}
    \includegraphics[width=\pairwidth]{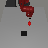}
    \includegraphics[width=\pairwidth]{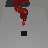}
    \includegraphics[width=\pairwidth]{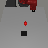}
    \includegraphics[width=\pairwidth]{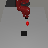}
    \includegraphics[width=\pairwidth]{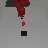}
    \includegraphics[width=\pairwidth]{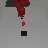}

    \caption{Example paired frames.  The paired frames were found by selecting frames where the puck and manipulator were in similar locations between the robot and the human data. Due to the differences in the morphologies of the agents, there are numerous instances where the human hand is in contact with the puck, while the robot manipulator is not in contact with the puck.}
    \label{fig:paired_frames}
\end{figure}
